# Supplementary material for: Transmission-line resonators for the study of individual two-level tunneling systems
Source: arXiv:1709.00381 ancillary file (2017-09-01)
Supplement: Supplementary file 1 [file supplementary.pdf]

Supplementary Material for

# Transmission-line resonators for the study of individual two-level tunneling systems

Jan David Brehm[1], Alexander Bilmes[1], Georg Weiss[1], Alexey V. Ustinov[1,2], and Jürgen Lisenfeld[1]

[1] *Physikalisches Institut, Karlsruhe Institute of Technology, 76131 Karlsruhe, Germany*
[2] *Russian Quantum Center, 100 Novaya St., Skolkovo, 143025 Moscow region, Russia*

July 25, 2017

## Input-Output theory of the cQED system

In order to understand the signature of a transmitted microwave signal in the one-photon limit that has interacted with a cQED system, one has to switch from a classical calculation of the S-Matrix to a quantum mechanical approach. As stated in the main article, a TLS that is coherently coupled to a photon mode of a resonator is described by the Jaynes-Cummings-Hamiltonian [1]. However, to probe such a system experimentally, the cavity has to be coupled to the measurement apparatus via a transmission line. In addition, both the two-level system and the cavity are dissipative and lose photons to the environment. The complete model which was considered in this work is depicted in Fig. S1. For better fits to the experimental data, we account for the mismatched feedline with a second cavity which represents an approximation of the cable resonances (compare references [2,3]).

To calculate the $S_{21}$-Matrix element for this system, we employ the framework of Input-Output theory [4]. Furthermore we use the methods described in references [2, 5–7], resulting in:

$$S_{21}(\omega) = 1 - \frac{i\frac{1}{2}\kappa}{\omega - \omega_1 + i\frac{\kappa}{2} + \frac{\delta^2(\omega_{\mathrm{TLS}} - \omega - i\frac{\Gamma_{\mathrm{TLS}}}{2})}{(\omega_2 - \omega - i\frac{\Gamma_{\mathrm{c}}}{2})(\omega_{\mathrm{TLS}} - \omega - i\frac{\Gamma_{\mathrm{TLS}}}{2}) - g^2}} \tag{S1}$$

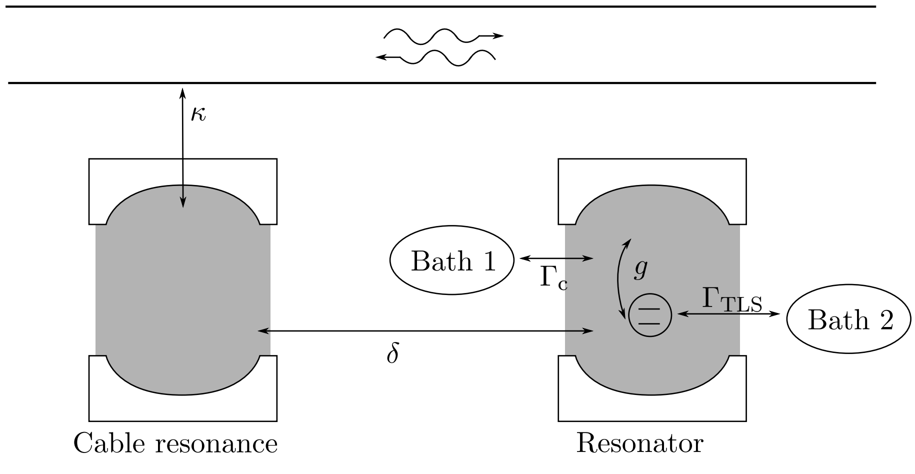


Supplementary Figure S1: Model used for analytical derivation of the $S_{21}$-matrix element within the framework of Input-Output theory.

In equation S1, $\omega_1$ and $\omega_2$ are the resonance frequencies of cable resonance and the actual resonator, $\kappa$, $\delta$ and $g$ are coupling rates and $\Gamma_{\mathrm{TLS}}$ and $\Gamma_{\mathrm{c}}$ are loss rates of TLS and cavity, respectively. This result is valid in the weak-excitation approximation, thus in the single photon-regime. Thermal excitation of TLS is neglected.

When fitting this formula to experimental data (compare Fig. 2c) in the main article) we first fit the background signal of the resonator without a strongly coupled TLS tuned in resonance (compare Fig. 2b) in the main article, fit not shown) to reduce the number of free parameters.

# Parameters of individual TLS

We fit the double-dip features of strongly coupled TLS in the measured $|S_{21}|$-Signal to the absolute value of equation (S1) and extract a TLS' resonance frequency $\omega_{\mathrm{TLS}}$, decoherence rate $\Gamma_{\mathrm{TLS}}$ and -time $T_2$, and TLS-resonator coupling strength $g$. We calculate the component of the TLS' electric dipole moment which is parallel to the electric field $p_{\|}$ using the fitted coupling strength $\hbar g = p_{\|} \cdot |E_{\mathrm{RMS}}|$ and the electric field strength in the capacitor $|E_{\mathrm{RMS}}|$ when the resonator is in its ground state. To obtain the electric field strength in the capacitor, we use SPICE to simulate the complete circuit including the transmission line and estimate the circuit parameters from the experimentally determined resonator quality factors in the one-photon regime. The obtained values are listed in table S1 with uncertainties corresponding to the confidence intervals of the fit. For the dipole moments, an additional uncertainty arises from the fit errors in the quality factors.

Table S1: Extracted fit parameters for strongly coupled TLS in resonator 3. The errors for the resonance frequency are smaller than $10^5$ Hz and thus not listed.

| TLS # | $\frac{\omega_{\mathrm{TLS}}}{2\pi}$ (GHz) | $\frac{\Gamma_{\mathrm{TLS}}}{2\pi}$ (MHz) | $\frac{g}{2\pi}$ (MHz) | $T_2$ (ns) | $p_{\|}$ (D) |
|---|---|---|---|---|---|
| 1 | 5.5853 | $0.49 \pm 0.1$ | $0.49 \pm 0.02$ | $323 \pm 62$ | $3.48 \pm 0.14$ |
| 2 | 5.5869 | $0.44 \pm 0.05$ | $0.48 \pm 0.02$ | $363 \pm 43$ | $3.40 \pm 0.14$ |
| 3 | 5.5859 | $0.54 \pm 0.08$ | $0.32 \pm 0.02$ | $296 \pm 46$ | $2.27 \pm 0.14$ |
| 4 | 5.5841 | $1.56 \pm 0.50$ | $1.04 \pm 0.15$ | $102 \pm 32$ | $7.39 \pm 1.06$ |
| 5 | 5.5844 | $0.84 \pm 0.10$ | $0.79 \pm 0.03$ | $189 \pm 22$ | $5.60 \pm 0.21$ |

# Deformation Potentials of individual TLS

The deformation potentials $\gamma$ of TLS can be obtained by fitting the hyperbolic dependence of TLS energies on the applied strain to the following equation:

$$E = \hbar\omega_{\mathrm{TLS}} = \sqrt{\Delta^2 + 4\gamma^2(\epsilon - \epsilon_0)^2} \tag{S2}$$

In Fig. S2 a) an extended range of the $|S_{21}|$-signal dependence of resonator 3 on strain is shown. The fits of equation (S2) to hyperbolic signatures of strongly coupled TLS for this measurement are depicted in Fig. S2 b). Analogously, hyperbolas found in the measurement of resonator 2 were fitted (not shown here). An overview of the extracted deformation potentials $\gamma$ is given in Fig. S3.

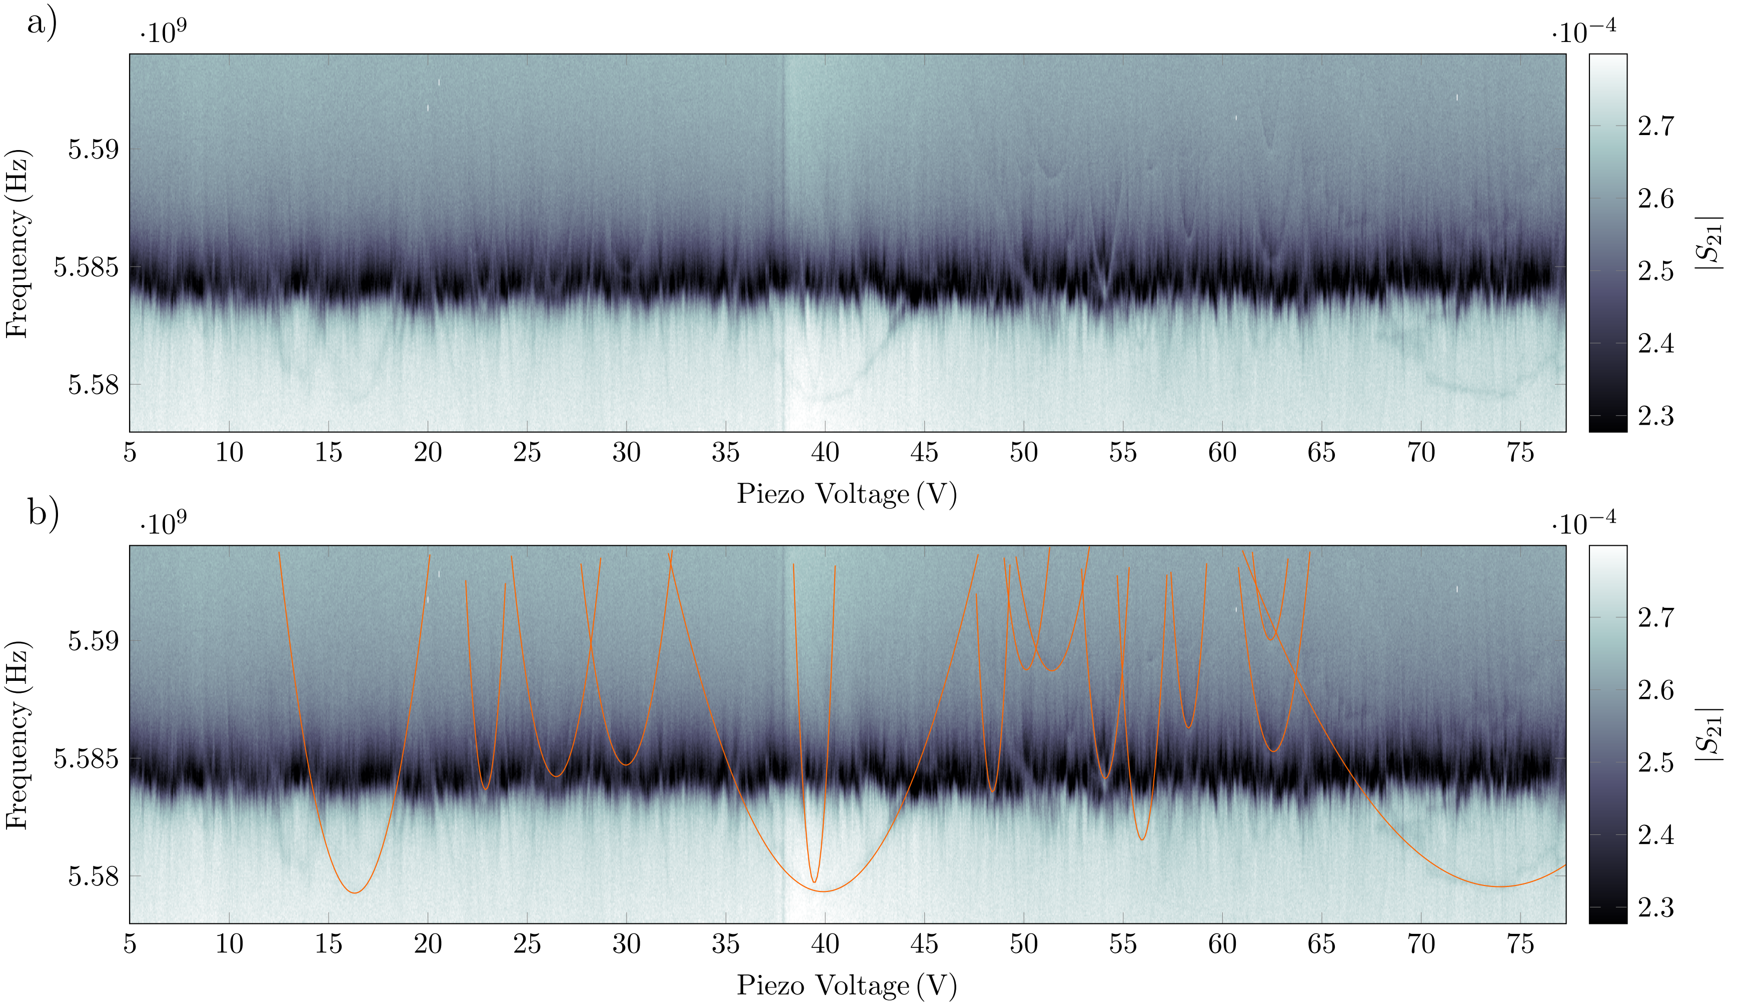


Supplementary Figure S2: a) Dependence of the $|S_{21}|$-signal of resonator 3 on strain. The shown data set is the same as in the main article, however an extended range is displayed. Several hyperbolas produced by strongly coupled TLS are visible. b) Fits of equation (S2) to visible hyperbolas. Only hyperbolas are fitted which have their symmetry points in the resonator bandwidth.

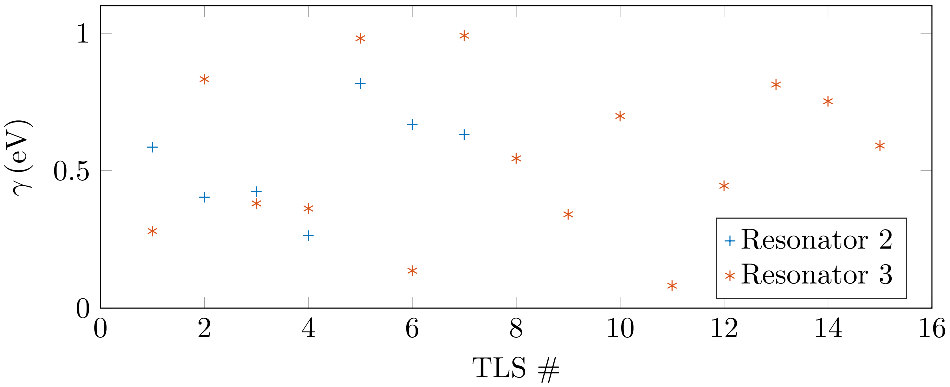


Supplementary Figure S3: Overview of deformation potentials of strongly coupled TLS found in resonator 2 and 3.

## References

[1] E.T. Jaynes and F.W. Cummings. Comparison of quantum and semiclassical radiation theories with application to the beam maser. *Proceedings of the IEEE*, 51(1):89–109, 1963.

[2] Bahman Sarabi. *Cavity Quantum Electrodynamics of Nanoscale Two-Level Systems*. Dissertation, University of Maryland, 2014.

[3] B. Sarabi, A. N. Ramanayaka, A. L. Burin, F. C. Wellstood, and K. D. Osborn. Cavity quantum electrodynamics using a near-resonance two-level system: Emergence of the glauber state. *Applied Physics Letters*, 106(17):172601, 2015.

[4] C. W. Gardiner and M. J. Collett. Input and output in damped quantum systems: Quantum stochastic differential equations and the master equation. *Phys. Rev. A*, 31:3761–3774, Jun 1985.

[5] Shanhui Fan, Ekin Kocabas, and Jung-Tsung Shen. Input-output formalism for few-photon transport in one-dimensional nanophotonic waveguides coupled to a qubit. *Phys. Rev. A*, 82:063821, Dec 2010.

[6] Eden Rephaeli and Shanhui Fan. Few-photon single-atom cavity qed with input-output formalism in fock space. *IEEE Journal of Selected Topics in Quantum Electronics*, 18(6):1754–1762, nov 2012.

[7] Eden Rephaeli and Shanhui Fan. Dissipation in few-photon waveguide transport, invited. *Photon. Res.*, 1(3):110–114, Oct 2013.
